# Supplementary material for: No Identity, no problem: Motion through detection for people tracking
Source: arXiv:2411.16466 source file (2024-11-25)
Supplement: Supplementary file 1 [file qualitative_supp.tex]

\begin{figure*}[h!]
    \centering
    \vspace{0.2cm}
    \includegraphics[width=0.91\linewidth]{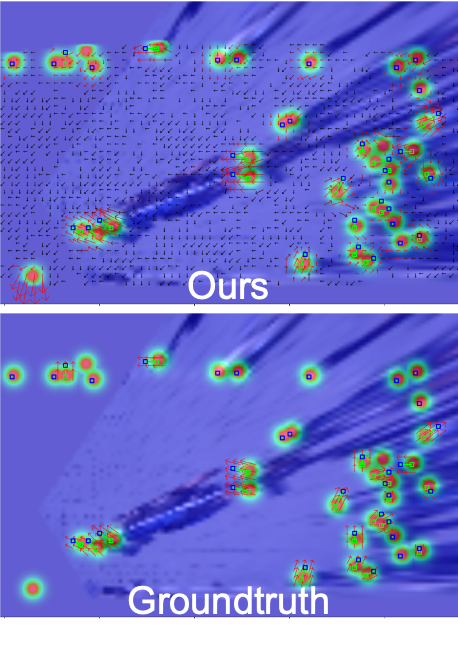}
    \caption{\textbf{Visualizing the Motion Offsets.} We visualize the detection and the motion offset predictions made by our model on top and the ground truth on the bottom. The green squares mark the position of the person at time $t$, and the blue squares indicate the position at time $t+1$. The green arrows, connecting these points, denote the ground truth motion. The offset map is visualized by regularly drawing arrows corresponding to the motion offsets. Qualitatively, the predicted detection and motion offsets appear very close to the ground truth ones.}
    \label{fig:qualitative_supp}
  \end{figure*}
